# Supplementary material for: Posner qubits: spin dynamics of entangled Ca$_9$(PO$_4$)$_6$ molecules and their role in neural processing
Source: arXiv:1807.06339 ancillary file (2018-07-17)
Supplement: Supplementary file 1 [file sup_info.pdf]

Supporting Information

# Posner qubits: spin dynamics of entangled $Ca_9(PO_4)_6$ molecules and their role in neural processing

Thomas C. Player and P. J. Hore

Department of Chemistry, University of Oxford, Oxford OX1 3QZ, UK

## 1 Spin Hamiltonian

For a pair of Posner molecules, the total spin Hamiltonian can be written as

$$\hat{H}(t) = \hat{H}_0 + \hat{H}_1(t), \tag{1}$$

where $\hat{H}_0$ describes coherent interactions, and $\hat{H}_1(t)$ describes time-dependent interactions that are responsible for relaxation of spin states. This can equivalently be written as a sum of smaller Hamiltonians for the individual molecules (which will be intermolecularly singlet entangled in Fisher's theory), labelled $a$ and $b$:

$$\hat{H}(t) = \hat{H}^a(t) \oplus \hat{H}^b(t) \tag{2}$$

where $\oplus$ denotes the Kronecker sum $\hat{A} \oplus \hat{B} = \hat{A} \otimes \hat{\mathbb{1}}_B + \hat{\mathbb{1}}_A \otimes \hat{B}$.

## 2 Coherent spin dynamics

The time-dependent singlet probability $p^{\mathrm{S}}_{j,k}(t)$, given an initial intermolecular singlet state $\hat{\rho}(0) = \hat{P}^{\mathrm{S}}_{a,b}/(Z_a Z_b)$ where $Z_i$ is a normalization constant to account for the other nuclear spin states in molecule $i$, is

$$\begin{aligned} p^{\mathrm{S}}_{j,k}(t) &= \mathrm{Tr}\left[\hat{\rho}(t)\hat{P}^{\mathrm{S}}_{a,b}\right] \\ &= \frac{1}{4} - \sum_{\beta=x,y,z} \mathrm{Tr}\left[\hat{\rho}(t)\hat{S}_{j\beta}\hat{S}_{k\beta}\right], \end{aligned} \tag{3}$$

where $\hat{\rho}(t) = \mathrm{e}^{-i\hat{H}_0 t}\hat{\rho}(0)\mathrm{e}^{+i\hat{H}_0 t}$ and $\hat{P}^{\mathrm{S}}_{j,k} = \frac{1}{4}\hat{\mathbb{1}} - \hat{\mathbf{S}}_j \cdot \hat{\mathbf{S}}_k$. This is time consuming to calculate in the full Hilbert space of two Posner molecules, and so we used a method for calculating time-dependent singlet probabilities of radical pairs in a smaller Hilbert space, described in [1, 2].

The second term in Eq. (3) can be rewritten using Eq. (2) and the fact that $\hat{H}^a(t)$ and $\hat{H}^b(t)$ commute as

$$-\frac{1}{Z_a Z_b}\sum_{\beta=x,y,z}\mathrm{Tr}\left[\mathrm{e}^{-i\hat{H}_0 t}\left(\frac{1}{4}\hat{\mathbb{1}}-\sum_{\alpha=x,y,z}\hat{S}_{a\alpha}\hat{S}_{b\alpha}\right)\mathrm{e}^{+i\hat{H}_0 t}\hat{S}_{j\beta}\hat{S}_{k\beta}\right]=\sum_{\alpha,\beta}R^{a,j}_{\alpha\beta}(t)R^{b,k}_{\alpha\beta}(t), \tag{4}$$

where

$$R^{a,j}_{\alpha\beta}(t)=\frac{1}{Z_a}\mathrm{Tr}\left[\hat{S}_{a\alpha}\mathrm{e}^{+i\hat{H}^a_0 t}\hat{S}_{j\beta}\mathrm{e}^{-i\hat{H}^a_0 t}\right]=\frac{1}{Z_a}\mathrm{Tr}\left[\hat{S}_{a\alpha}(0)\hat{S}_{j\beta}(t)\right] \tag{5}$$

is an element of the spin correlation tensor for the chosen nucleus in molecule $a$, and we have used cyclic permutation under the trace.

Using Eqs (3) and (4), we can therefore calculate the time-dependent singlet probability in the smaller Hilbert space of each individual molecule as

$$p^{\mathrm{S}}_{j,k}(t)=\frac{1}{4}+\sum_{\alpha,\beta}R^{a,j}_{\alpha\beta}(t)R^{b,k}_{\alpha\beta}(t). \tag{6}$$

# 3 Concurrence

The concurrence between two spins was calculated by first tracing out the other ten spins in the two-molecule system from the density matrix to give $\rho(t)=\mathrm{Tr}_{i\neq\{j,k\}}\left[\hat{\rho}(t)\right]$ [1]. The concurrence was then calculated as in [4]:

$$C_{j,k}(t)=\max\{0,\lambda_1-\lambda_2-\lambda_3-\lambda_4\}, \tag{7}$$

where $\lambda_i$ are the eigenvalues, in decreasing order, of the matrix $\rho(t)\,(\sigma_y\otimes\sigma_y)\,\rho(t)\,(\sigma_y\otimes\sigma_y)$ and $\sigma_y$ is the second Pauli matrix. This concurrence, which has range 0 (not entangled) to 1 (fully entangled), can then be used directly as a measure of bipartite entanglement.

# 4 Validity of the Redfield approach

The dominant relaxation pathway for many molecules containing non-quadrupolar nuclei is dipolar relaxation via the interaction of nuclear magnetic moments in the molecule. Note that this is intramolecular dipolar coupling, as opposed to the intermolecular dipolar coupling considered by Fisher and colleagues [5, 6]. Brownian rotational diffusion of the molecule then modulates these dipolar couplings and leads to relaxation. We use Redfield theory to model this kind of spin relaxation. The validity of the Redfield approach used can be established from the following estimates.

(1) For the Redfield approach to be valid, we require $|b|\tau_{\mathrm{c}}\ll 1$ [7, 8]. In this expression $b$ is the dipolar coupling constant of two $^{31}$P spins separated by a distance $r$, defined as $b=-(4\pi r^3)^{-1}\mu_0\gamma_{\mathrm{P}}^2\hbar$, where $\gamma_{\mathrm{P}}$ is the magnetogyric ratio of $^{31}$P and $\mu_0$ is the vacuum permeability. Taking $r=0.5\,\mathrm{nm}$ as a rough figure for the average separation of the $^{31}$P nuclei, we obtain $b\simeq 990\,\mathrm{Hz}$. The correlation time for Brownian rotation diffusion of a spherical molecule of radius $a$ in a medium with viscosity $\eta$ at temperature $T$ can be estimated using the Stokes–Einstein equation as $\tau_{\mathrm{c}}=4\pi\eta a^3(3k_BT)^{-1}$. Using $a=0.44\,\mathrm{nm}$ [9] and $T=310\,\mathrm{K}$ (physiological temperature), $\tau_{\mathrm{c}}\simeq 58\,\mathrm{ps}$ for water ($\eta=0.69\,\mathrm{mPa\,s}$). Multiplying by the dipolar coupling constant calculated above, we see that the Redfield approach is clearly valid.

[1] The code used for the partial trace can be found online at [3].

(2) To simplify the calculation further we use the extreme narrowing limit, as described in [10], which is valid when all the eigenvalue differences of the time-independent part of the spin Hamiltonian $\hat{H}_0$ are much smaller than $\tau_c^{-1}$. In the present case, since the $J$-couplings are small compared to the Earth's magnetic field, this means we require $6|\omega_0|\tau_c \ll 1$, where $\omega_0 = -\gamma_P B_0$ is the $^{31}$P nuclear Larmor frequency in the Earth's magnetic field $B_0$. Taking $B_0 \simeq 50\,\mu$T, $\omega_0 \simeq 5.4\,$kHz and so the extreme narrowing condition is clearly satisfied for the rotational correlation time quoted above. We also note that the six $^{31}$P nuclei in a Posner's molecule would have the same chemical shift since they are magnetically equivalent, and so the $^{31}$P NMR spectrum would be a singlet.

These two conditions establish that the extreme narrowing Redfield approach to calculating nuclear spin relaxation, as described elsewhere in [7, 10–14] and below, will be valid for Posner's molecules.

# 5 Dipolar Hamiltonian

The following description of the dipolar Hamiltonian follows that described by Wagner-Rundell [10] and the references therein.

If we define the the dipole-dipole axis as the principal axis frame (P) $z$-axis, then the Hamiltonian for dipolar coupling in a molecule between nuclei $j$ and $k$ is given by

$$\hat{H}_D^{jk(\mathrm{P})} = \sqrt{6} b_{jk} \hat{T}_{2,0}^{jk}, \tag{8}$$

where $b_{jk} = -\frac{1}{4\pi}\mu_0 \gamma_j \gamma_k \hbar r_{jk}^{-3}$ is the dipole-dipole coupling constant, $\mu_0$ is the vacuum permeability, $r_{jk}$ is the internuclear distance, and $\hat{T}_{2,0}^{jk}$ is one of the second-order spherical tensors:

$$\begin{gathered} \hat{T}_{2,\pm2}^{jk} = \tfrac{1}{2}\hat{S}_{j\pm}\hat{S}_{k\pm} \quad , \quad \hat{T}_{2,\pm1}^{jk} = \mp\tfrac{1}{2}\left(\hat{S}_{jz}\hat{S}_{k\pm} + \hat{S}_{j\pm}\hat{S}_{kz}\right), \\ \hat{T}_{2,0}^{jk} = \sqrt{\tfrac{2}{3}}\left(-\tfrac{1}{2}\hat{S}_{jx}\hat{S}_{kx} - \tfrac{1}{2}\hat{S}_{jy}\hat{S}_{ky} + \hat{S}_{jz}\hat{S}_{kz}\right). \end{gathered} \tag{9}$$

Any spherical tensor is transformed under a rotation operator $\hat{\hat{R}}$ as

$$\hat{\hat{R}}(\alpha,\beta,\gamma)\hat{T}_{l,m}^{jk} = \sum_{m'=-l}^{l} \hat{T}_{l,m'}^{jk} \mathfrak{D}_{m',m}^{(l)}(\alpha,\beta,\gamma), \tag{10}$$

where $\mathfrak{D}_{m',m}^{(l)}(\alpha,\beta,\gamma)$ are elements of the $l^{\text{th}}$ rank Wigner D-matrix for a rotation through Euler angles $(\alpha,\beta,\gamma)$. [2]

This leads to the following expression for the dipolar Hamiltonian in the laboratory frame (L), where it has been rotated from the principal axis frame to the molecular frame through Euler angles

[2] The convention used here is the $z$-$y'$-$z''$ convention. The first rotation is of an angle $\alpha$ about the rotating object's $z$ axis, then $\beta$ about the new $y'$ axis, and finally $\gamma$ about the new $z''$ axis. This can also be written as $\hat{\hat{R}}(\alpha,\beta,\gamma) = \hat{\hat{R}}_{z''}(\gamma)\hat{\hat{R}}_{y'}(\beta)\hat{\hat{R}}_z(\alpha)$, in terms of the three separate rotations. This is equivalent to performing all three rotations in a different order about the original axes: $\hat{\hat{R}}(\alpha,\beta,\gamma) = \hat{\hat{R}}_z(\alpha)\hat{\hat{R}}_y(\beta)\hat{\hat{R}}_z(\gamma)$.

$(\alpha, \beta, \gamma)$, and then into the lab frame through time-dependent Euler angles $(\Omega\,(t))$:

$$\begin{aligned}\hat{H}_D^{jk\,(\mathrm{L})} &= \hat{\hat{R}}_{\mathrm{mol}}\left(\Omega\,(t)\right)\hat{\hat{R}}^{j,k}_{\mathrm{pos}}(\alpha,\beta,\gamma)\hat{H}_D^{jk\,(\mathrm{P})} \\ &= \hat{\hat{R}}_{\mathrm{mol}}\left(\Omega\,(t)\right)\hat{\hat{R}}^{j,k}_{\mathrm{pos}}(\alpha,\beta,\gamma)\sqrt{6}b_{jk}\hat{T}^{jk}_{2,0} \\ &= -\sqrt{6}\hbar\gamma_{\mathrm{P}}^2\left(\frac{\mu_0}{4\pi}\right)\hat{\hat{R}}_{\mathrm{mol}}\left(\Omega\,(t)\right)\hat{\hat{R}}^{j,k}_{\mathrm{pos}}(\alpha,\beta,\gamma)\hat{T}^{jk}_{2,0}/r^3_{jk}.\end{aligned} \tag{11}$$

The time-dependent Hamiltonian is then given by summing over all pairs of nuclei in the molecule (Eq. (2.2) in the main text):

$$\hat{H}_1(t) = -\sqrt{6}\hbar\gamma_{\mathrm{P}}^2\left(\frac{\mu_0}{4\pi}\right)\hat{\hat{R}}_{\mathrm{mol}}\left(\Omega\,(t)\right)\sum_{j<k}\sum_{k}\hat{\hat{R}}^{j,k}_{\mathrm{pos}}(\alpha,\beta,\gamma)\hat{T}^{jk}_{2,0}/r^3_{jk}. \tag{12}$$

We can evaluate the effect of the rotation operators on the spherical tensors using Eq. (10), and by defining a positioning parameter $\Phi^{jk}_m = \sqrt{6}b_{jk}\mathfrak{D}^{(2)}_{m,0}\left(\alpha,\beta,\gamma\right)$ for each pair of nuclei in the molecule can write the time-dependent Hamiltonian as

$$\hat{H}_1(t) = \sum_{j<k}\sum_{k}\sum_{m,m'=-2}^{2}\Phi^{jk}_m\hat{T}^{jk}_{2,m'}\mathfrak{D}^{(2)}_{m',m}\left(\Omega(t)\right). \tag{13}$$

This can be made notationally more compact by defining a parameter, $\phi^{jk}_{m'}(t)$, containing all time-dependent positional information about a pair of nuclei:

$$\phi^{jk}_{m'}(t) = \sum_{m=-2}^{2}\Phi^{jk}_m\mathfrak{D}^{(2)}_{m',m}\left(\Omega(t)\right), \tag{14}$$

such that the time-dependent Hamiltonian can be written as

$$\hat{H}_1(t) = \sum_{j<k}\sum_{k}\sum_{m'=-2}^{2}\phi^{jk}_{m'}(t)\hat{T}^{jk}_{2,m'}, \tag{15}$$

in a form that facilitates fast calculations.

# 6 Relaxation Theory

Relaxation due to $\hat{H}_1(t)$ can be described using a well-established theory often called Redfield, or Bloch-Redfield-Wangsness, relaxation theory.

The Liouville-von Neumann equation is used to determine the effect of the spin Hamiltonian on the system:

$$\frac{\mathrm{d}\hat{\rho}(t)}{\mathrm{d}t} = -i\left[\hat{H}_0 + \hat{H}_1(t), \hat{\rho}(t)\right]. \tag{16}$$

It is shown in [10] and [7] that, using second order perturbation theory and several valid assumptions, that this can be rewritten in the interaction representation. This is indicated by a double dagger (‡), whereby all operators in the laboratory frame are transformed according to

$$\hat{Q}^{\ddagger}(t) = \mathrm{e}^{i\hat{H}_0 t}\hat{Q}\mathrm{e}^{-i\hat{H}_0 t}. \tag{17}$$

In this representation, the time-evolution of the density matrix is given by

$$\frac{\mathrm{d}\hat{\rho}^{\ddagger}(t)}{\mathrm{d}t} = -\int_0^{\infty} \left\langle \left[\hat{H}_1^{\ddagger}(t), \left[\hat{H}_1^{\ddagger}(t-\tau), \hat{\rho}^{\ddagger}(t)\right]\right]\right\rangle \mathrm{d}\tau, \tag{18}$$

where the ensemble average is over the Hamiltonians. This expression is transformed back out of the interaction representation and into the laboratory frame using Eq. (17):

$$\frac{\mathrm{d}\hat{\rho}(t)}{\mathrm{d}t} = -i\left[\hat{H}_0, \hat{\rho}(t)\right] - \int_0^{\infty} \left\langle \left[\hat{H}_1(t), \left[\mathrm{e}^{-i\hat{H}_0\tau}\hat{H}_1(t-\tau)\mathrm{e}^{i\hat{H}_0\tau}, \hat{\rho}(t)\right]\right]\right\rangle \mathrm{d}\tau. \tag{19}$$

This is clearly a sum of two terms: the first governs the coherent dynamics of the system, which have already been discussed, and the second is the relaxation term. This is known as a "master equation".

# 7 Extreme Narrowing

This master equation is not analytically soluble in general, and so an approximation is outlined here, as in [10]. When the random processes (i.e. molecular rotations) take place on a timescale much shorter than all of the eigenvalue differences for the static Hamiltonian (i.e. the transition frequencies), then the conditions for extreme narrowing are met:

$$\omega_{nm}^2 \tau_{\mathrm{c}}^2 \ll 1 \quad \forall \quad n, m, \tag{20}$$

where $\tau_{\mathrm{c}}$ is the molecular rotational correlation time, i.e. the average time for a molecule to tumble through an angle of one radian, and $\omega_{nm} = \omega_n - \omega_m$ where $\{\omega_n\}$ are the eigenvalues of $\hat{H}_0$.

By converting into the eigenbasis of $\hat{H}_0$, the relaxation term in Eq. (19) can be written

$$-\left(\int_0^{\infty} \left\langle \left[\hat{H}_1^{(0)}(t), \left[\hat{F}(t,\tau), \hat{\rho}^{(0)}(t)\right]\right]\right\rangle \mathrm{d}\tau\right), \tag{21}$$

where $\hat{F}(t,\tau) = \mathrm{e}^{-i\hat{H}_0^{(0)}\tau}\hat{H}_1^{(0)}(t-\tau)\mathrm{e}^{i\hat{H}_0^{(0)}\tau}$, and the (0) superscript indicates quantities transformed into the new basis.

Expanding the commutators, remembering that the ensemble average is taken only over the time-dependent Hamiltonian, means that terms similar to $\hat{K}$ arise:

$$\hat{K} = \int_0^{\infty} \left\langle \hat{H}_1^{(0)}(t)\hat{F}(t,\tau)\right\rangle \hat{\rho}^{(0)}(t)\mathrm{d}\tau. \tag{22}$$

A single matrix element of $\hat{K}$ can be written as

$$\begin{aligned} \hat{K}_{nm} &= \sum_{p,q}\int_0^{\infty} \left\langle \left[\hat{H}_1^{(0)}(t)\right]_{np}\left[\hat{F}(t,\tau)\right]_{pq}\right\rangle \left[\hat{\rho}^{(0)}(t)\right]_{qm}\mathrm{d}\tau \\ &= \sum_{p,q}\int_0^{\infty} \left\langle \left[\hat{H}_1^{(0)}(t)\right]_{np}\left[\hat{H}_1^{(0)}(t-\tau)\right]_{pq}\right\rangle \left[\hat{\rho}^{(0)}(t)\right]_{qm}\mathrm{e}^{-i\omega_{pq}\tau}\mathrm{d}\tau. \end{aligned} \tag{23}$$

Using the correlation function

$$\left\langle \hat{H}_1(t)\hat{H}_1(t-\tau)\right\rangle = \left\langle \hat{H}_1(t)\hat{H}_1(t)\right\rangle \mathrm{e}^{-\frac{|\tau|}{\tau_{\mathrm{c}}}}, \tag{24}$$

where the angle brackets indicate an ensemble average, gives:

$$\hat{K}_{nm} = \sum_{p,q} \int_0^\infty \left\langle \left[\hat{H}_1^{(0)}(t)\right]_{np} \left[\hat{H}_1^{(0)}(t)\right]_{pq} \right\rangle \left[\hat{\rho}^{(0)}(t)\right]_{qm} \mathrm{e}^{(-i\omega_{pq} - \frac{1}{\tau_c})\tau} \mathrm{d}\tau. \tag{25}$$

This integral is simple to compute, and gives:

$$\hat{K}_{nm} = \sum_{p,q} \left\langle \left[\hat{H}_1^{(0)}(t)\right]_{np} \left[\hat{H}_1^{(0)}(t)\right]_{pq} \right\rangle \left[\hat{\rho}^{(0)}(t)\right]_{qm} \left( \frac{\tau_c}{1+\tau_c^2\omega_{pq}^2} - i\frac{\omega_{pq}\tau_c^2}{1+\tau_c^2\omega_{pq}^2} \right), \tag{26}$$

the imaginary component of which is known as the dynamic frequency shift. It corresponds to a shift in energy which is usually small and difficult to measure, and so we ignore it here [8].

Since we are in the extreme narrowing limit, $\tau_c/(1+\tau_c^2\omega_{pq}^2) \simeq \tau_c$, and so:

$$\hat{K}_{nm} \simeq \tau_c \sum_{p,q} \left\langle \left[\hat{H}_1^{(0)}(t)\right]_{np} \left[\hat{H}_1^{(0)}(t)\right]_{pq} \right\rangle \left[\hat{\rho}^{(0)}(t)\right]_{qm}. \tag{27}$$

Using a similar argument for all terms in Eq. (21) means we obtain the relaxation term in the extreme narrowing limit:

$$-\tau_c \left\langle \left[\hat{H}_1^{(0)}(t), \left[\hat{H}_1^{(0)}(t), \hat{\rho}^{(0)}(t)\right]\right] \right\rangle. \tag{28}$$

So, by transforming back out of the eigenbasis of $\hat{H}_0$, we obtain the master equation in the extreme narrowing limit:

$$\frac{\mathrm{d}\hat{\rho}(t)}{\mathrm{d}t} = -i\left[\hat{H}_0, \hat{\rho}(t)\right] - \tau_c \left\langle \left[\hat{H}_1(t), \left[\hat{H}_1(t), \hat{\rho}(t)\right]\right] \right\rangle. \tag{29}$$

# 8 Relaxation Superoperator

The time-dependence of the density matrix can also be written using in Liouville space [3] as

$$\frac{\mathrm{d}\left|\hat{\rho}(t)\right\rangle}{\mathrm{d}t} = \left(-i\hat{\hat{H}}_0 + \hat{\hat{\Gamma}}\right)\left|\hat{\rho}(t)\right\rangle, \tag{30}$$

where $\hat{\hat{H}}_0$ is the commutation superoperator that corresponds to $\hat{H}_0$, and $\hat{\hat{\Gamma}}$ is the relaxation superoperator:

$$\hat{\hat{\Gamma}} = -\left\langle \hat{\hat{H}}_1(t)\hat{\hat{H}}_1(t) \right\rangle \tau_c. \tag{31}$$

Using Eq. (12), the relaxation superoperator may be written:

$$\hat{\hat{\Gamma}} = -\tau_c \left\langle \sum_{j<k}\sum_{k}\sum_{r<s}\sum_{s}\sum_{m',n'=-2}^{2} \phi_{m'}^{jk}(t)\phi_{n'}^{rs}(t)\hat{\hat{T}}_{2,m'}^{jk}\hat{\hat{T}}_{2,n'}^{rs} \right\rangle. \tag{32}$$

Since the time-dependence comes from the positioning $\phi(t)$ functions, it is sufficient to consider products of the form:

$$\left\langle \phi_{m'}^{jk}(t)\phi_{n'}^{rs}(t) \right\rangle. \tag{33}$$

[3] This is where density matrices are row-wise flattened into Liouville space state "vectors" that are acted upon by matrix representations of superoperators of the dimension of the Hilbert space squared.

Using Eq. (14) and the properties of Wigner functions [4], products of this type can be expressed as:

$$\begin{aligned}\left\langle \phi^{jk}_{m'}(t)\phi^{rs}_{n'}(t)\right\rangle &= \sum_{m,n=-2}^{2} \Phi^{jk}_{m}\Phi^{rs}_{n}\left\langle \mathfrak{D}^{(2)}_{m',m}\left(\Omega(t)\right)\mathfrak{D}^{(2)}_{n',n}\left(\Omega(t)\right)\right\rangle \\ &= \sum_{m,n=-2}^{2} \Phi^{jk}_{m}\Phi^{rs}_{n}\left\langle \mathfrak{D}^{(2)}_{m',m}\left(\Omega(t)\right)\mathfrak{D}^{*(2)}_{-n',-n}\left(\Omega(t)\right)\right\rangle (-1)^{m'-m}.\end{aligned} \tag{34}$$

From [10]:

$$\begin{aligned}\left\langle \phi^{jk}_{m'}(t)\phi^{rs}_{n'}(t)\right\rangle &= \frac{1}{5}\sum_{m,n=-2}^{2} \Phi^{jk}_{m}\Phi^{rs}_{n}\delta_{m',-n'}\ \delta_{m,-n}(-1)^{m'-m} \\ &= \frac{1}{5}\sum_{m=-2}^{2} \Phi^{jk}_{m}\Phi^{rs}_{-m}\delta_{m',-n'}(-1)^{m'-m}.\end{aligned} \tag{35}$$

The relaxation superoperator in the extreme narrowing limit can therefore be calculated directly as:

$$\hat{\hat{\Gamma}} = -\frac{\tau_{\mathrm{c}}}{5}\sum_{j<k}\sum_{k}\sum_{r<s}\sum_{s}\sum_{n,m=-2}^{2}(-1)^{n+m}\Phi^{jk}_{m}\Phi^{rs}_{-m}\hat{\hat{T}}^{jk}_{2,-n}\hat{\hat{T}}^{rs}_{2,n}. \tag{36}$$

We now consider the effect of $\hat{\hat{\Gamma}}$ on the intermolecular singlet state. The self-relaxation rate constant $\Gamma_{\mathrm{S}}$ for this state is given as in [13] and the main text by

$$\Gamma_{\mathrm{S}} = \frac{\mathrm{Tr}\left[\left(\hat{\hat{\Gamma}}\,|\hat{P}^{\mathrm{S}}_{a,b}\rangle\right)\hat{P}^{\mathrm{S}}_{a,b}\right]}{\mathrm{Tr}\left[\hat{P}^{\mathrm{S}}_{a,b}\hat{P}^{\mathrm{S}}_{a,b}\right]} = \mathrm{Tr}\left[\hat{P}^{\mathrm{S}}_{a,b}\hat{\hat{\Gamma}}\hat{P}^{\mathrm{S}}_{a,b}\right]/\mathrm{Tr}\left[\hat{P}^{\mathrm{S}}_{a,b}\hat{P}^{\mathrm{S}}_{a,b}\right], \tag{37}$$

where $a$ and $b$ are the two entangled spins in the singlet state.

# 9 Relaxation of an Intermolecular Singlet

Using Eq.s (29) and (31) and the definition of $\hat{P}^{\mathrm{S}}_{a,b}$, the unnormalized initial singlet relaxation rate constant $\Gamma'_{\mathrm{S}}$ can be written (in units of $-\tau_{\mathrm{c}}$) as:

$$\begin{aligned}\Gamma'_{\mathrm{S}} &= \mathrm{Tr}\left[\left\langle\left[\hat{H}_1(t),\left[\hat{H}_1(t),\hat{P}^{\mathrm{S}}_{a,b}\right]\right]\right\rangle\hat{P}^{\mathrm{S}}_{a,b}\right] \\ &= \mathrm{Tr}\left[\left\langle\left[\hat{H}_1(t),\left[\hat{H}_1(t),\frac{1}{4}\mathbb{1}-\sum_{\alpha}\hat{S}_{a\alpha}\otimes\hat{S}_{b\alpha}\right]\right]\right\rangle\frac{1}{4}\mathbb{1}-\sum_{\beta}\hat{S}_{a\beta}\otimes\hat{S}_{b\beta}\right] \\ &= \sum_{\alpha,\beta}\mathrm{Tr}\left[\left\langle\left[\hat{H}_1(t),\left[\hat{H}_1(t),\hat{S}_{a\alpha}\otimes\hat{S}_{b\alpha}\right]\right]\right\rangle\hat{S}_{a\beta}\otimes\hat{S}_{b\beta}\right] \\ &= \sum_{\alpha,\beta}\mathrm{Tr}\left[\left\langle\left[\hat{H}_1(t),\left[\hat{H}_1(t),\hat{S}_{a\alpha}\otimes\hat{S}_{b\alpha}\right]\right]\right\rangle\hat{S}_{a\beta}\otimes\hat{S}_{b\beta}\right] \\ &= \sum_{\alpha,\beta}\mathrm{Tr}\left[\langle\mathrm{A}\rangle\,\hat{S}_{a\beta}\otimes\hat{S}_{b\beta}\right].\end{aligned} \tag{38}$$

[4]Specifically, $\mathfrak{D}^{(j)}_{m',m}(\alpha,\beta,\gamma) = (-1)^{m'-m}\mathfrak{D}^{*(j)}_{-m',-m}(\alpha,\beta,\gamma)$.

The term labelled A can then be written, using Eq. (2) and expanding the commutators, as

$$\begin{aligned}
\mathrm{A} &= \left[\hat{H}_1^a(t) \oplus \hat{H}_1^b(t), \left[\hat{H}_1^a(t) \oplus \hat{H}_1^b(t), \hat{S}_{a\alpha} \otimes \hat{S}_{b\alpha}\right]\right] \\
&= \left[\hat{H}_1^a(t), \left[\hat{H}_1^a(t), \hat{S}_{a\alpha}\right]\right] \otimes \hat{S}_{b\alpha} + 2\left[\hat{H}_1^a(t), \hat{S}_{a\alpha}\right] \otimes \left[\hat{H}_1^b(t), \hat{S}_{b\alpha}\right] \\
&\quad + \hat{S}_{a\alpha} \otimes \left[\hat{H}_1^b(t), \left[\hat{H}_1^b(t), \hat{S}_{b\alpha}\right]\right].
\end{aligned} \tag{39}$$

The second term of the last expression will be zero under an ensemble average since the tumbling of the two molecules is uncorrelated. We note that the commutators in Eq. (39) are of the same form as those in Eq. (31), and so we define a relaxation superoperator for each separate molecule,

$$\hat{\hat{\Gamma}}^i = -\left\langle \hat{\hat{H}}_1^i(t)\hat{\hat{H}}_1^i(t) \right\rangle \tau_\mathrm{c}, \tag{40}$$

such that Eq. (38) can now be written as

$$\begin{aligned}
\Gamma'_\mathrm{S} &= \sum_{\alpha,\beta} \mathrm{Tr}\left[\left(\left(\hat{\hat{\Gamma}}^a \,|\hat{S}_{a\alpha}\rangle\right) \otimes \hat{S}_{b\alpha} + \hat{S}_{a\alpha} \otimes \left(\hat{\hat{\Gamma}}^b \,|\hat{S}_{b\alpha}\rangle\right)\right)\left(\hat{S}_{a\beta} \otimes \hat{S}_{b\beta}\right)\right] \\
&= \sum_{\alpha,\beta} \mathrm{Tr}\left[\left(\hat{\hat{\Gamma}}^a \,|\hat{S}_{a\alpha}\rangle\right)\hat{S}_{a\beta} \otimes \hat{S}_{b\alpha}\hat{S}_{b\beta} + \hat{S}_{a\alpha}\hat{S}_{a\beta} \otimes \left(\hat{\hat{\Gamma}}^b \,|\hat{S}_{b\alpha}\rangle\right)\hat{S}_{b\beta}\right] \\
&= \sum_{\alpha,\beta} \mathrm{Tr}\left[\left(\hat{\hat{\Gamma}}^a \,|\hat{S}_{a\alpha}\rangle\right)\hat{S}_{a\beta}\right] \mathrm{Tr}\left[\hat{S}_{b\alpha}\hat{S}_{b\beta}\right] + \mathrm{Tr}\left[\hat{S}_{a\alpha}\hat{S}_{a\beta}\right] \mathrm{Tr}\left[\left(\hat{\hat{\Gamma}}^b \,|\hat{S}_{b\alpha}\rangle\right)\hat{S}_{b\beta}\right] \\
&= \sum_{\alpha} 2^{N_a-2}\mathrm{Tr}\left[\left(\hat{\hat{\Gamma}}^a \,|\hat{S}_{a\alpha}\rangle\right)\hat{S}_{a\alpha}\right] + 2^{N_b-2}\mathrm{Tr}\left[\left(\hat{\hat{\Gamma}}^b \,|\hat{S}_{b\alpha}\rangle\right)\hat{S}_{b\alpha}\right],
\end{aligned} \tag{41}$$

using the fact that $\mathrm{Tr}\left[\hat{S}_{ip}\hat{S}_{iq}\right] = 2^{N_i-2}\delta_{pq}$, where $N_i$ is the number of spins in a molecule, $i$. Therefore, the singlet relaxation rate constant can be calculated as

$$\Gamma'_\mathrm{S} = \sum_{i}^{a,b} 2^{N_i-2} \sum_{\alpha}^{x,y,z} \mathrm{Tr}\left[\hat{S}_{i\alpha}\hat{\hat{\Gamma}}^i\hat{S}_{i\alpha}\right] / \mathrm{Tr}\left[\hat{P}^\mathrm{S}_{a,b}\hat{P}^\mathrm{S}_{a,b}\right], \tag{42}$$

with the relaxation superoperators each in the Liouville space of just one molecule, rather than of the whole system. By comparison with Eq. (37), it can be seen that this is a sum of the self relaxation rates for each Cartesian component of the singlet state.

In general $\hat{\hat{\Gamma}}^1 \neq \hat{\hat{\Gamma}}^2$, since the two molecules in the intermolecular singlet state could be different, but in our case the two molecules are identical and so $\hat{\hat{\Gamma}}^1 = \hat{\hat{\Gamma}}^2 = \hat{\hat{\Gamma}}'$, further simplifying the calculation:

$$\Gamma'_\mathrm{S} = 2^{N-1} \sum_{\alpha}^{x,y,z} \mathrm{Tr}\left[\hat{S}_{i\alpha}\hat{\hat{\Gamma}}'\hat{S}_{i\alpha}\right] / \mathrm{Tr}\left[\hat{P}^\mathrm{S}_{a,b}\hat{P}^\mathrm{S}_{a,b}\right]. \tag{43}$$

# 10 DFT Results

Table 1 shows the DFT optimized atomic coordinates of an $S_6$ Posner molecule.These were obtained by optimizing the geometry for a Posner molecule with $S_6$ symmetry from [15] in Gaussian 09

using density functional theory (DFT). The Ahlrich triple-zeta basis set def2-TZVPP was used in combination with the BP86 functional. The DFT work was performed by Daniel Kattnig (now at the Living Systems Institute, University of Exeter, UK).

## References


[1] K. Schulten and P. G. Wolynes, J. Chem. Phys. **68**, 3292 (1978).

[2] D. E. Manolopoulos and P. J. Hore, J. Chem. Phys. **139**, 124106 (2013).

[3] T. Cubitt, "Dr. Qubit," (2018).

[4] W. K. Wootters, Phys. Rev. Lett. **80**, 2245 (1998).

[5] M. P. A. Fisher, Ann. Phys. **362**, 593 (2015).

[6] M. W. Swift, C. G. Van de Walle, and M. P. A. Fisher, Phys. Chem. Chem. Phys. **20**, 12373 (2018).

[7] M. Goldman, J. Magn. Reson. **149**, 160 (2001).

[8] J. H. Freed and G. K. Fraenkel, J. Chem. Phys. **39**, 326 (1963).

[9] A. Dey, P. H. H. Bomans, F. A. Muller, J. Will, P. M. Frederik, G. de With, and N. A. J. M. Sommerdijk, Nat. Mater. **9**, 1010 (2010).

[10] N. Wagner-Rundell, *Electron Spin Relaxation Effects on Radical Recombination Reactions in Weak Magnetic Fields*, Ph.D. thesis, University of Oxford (2008).

[11] A. G. Redfield, Adv. Magn. Reson. **1**, 1 (1965).

[12] C. P. Slichter, *Principles of Magnetic Resonance* (Springer-Verlag, Berlin, 1978).

[13] I. Kuprov, N. Wagner-Rundell, and P. J. Hore, J. Magn. Reson. **184**, 196 (2007).

[14] S. Worster, D. R. Kattnig, and P. Hore, J. Chem. Phys. **145**, 035104 (2016).

[15] G. Treboux, P. Layrolle, N. Kanzaki, K. Onuma, and A. Ito, J. Phys. Chem. A **104**, 5111 (2000).

Table 1: DFT optimized atomic coordinates, in Å, for Posner's molecule with $S_6$ symmetry. Numbering of the phosphorus nuclei is as in Fig. 1, main text.

| | | $x$ | $y$ | $z$ |
|---|---|---|---|---|
| 1 | O | −0.9344 | +3.8163 | +1.4609 |
| 2 | Ca | −2.7835 | +2.0443 | +0.7842 |
| 3 | O | −1.7198 | +2.5381 | −1.1499 |
| 4 | Ca | +0.3786 | +3.4328 | −0.7842 |
| 5 | O | −3.7722 | +1.0989 | −1.4609 |
| 6 | P(1) | +0.0000 | +2.6944 | +2.0654 |
| 7 | P(5) | −2.3334 | +1.3472 | −2.0654 |
| 8 | O | −1.9765 | +1.4995 | −3.5593 |
| 9 | O | +0.3104 | +2.4615 | +3.5593 |
| 10 | O | +1.3382 | +2.7585 | +1.1499 |
| 11 | O | −0.8317 | +1.3528 | +1.6409 |
| 12 | O | +2.8378 | +2.7174 | −1.4609 |
| 13 | O | −3.0580 | −0.2203 | +1.1499 |
| 14 | O | +0.7557 | +1.3966 | −1.6409 |
| 15 | O | −1.5874 | −0.0439 | −1.6409 |
| 16 | P(4) | +2.3334 | +1.3472 | −2.0654 |
| 17 | Ca | −3.1622 | −1.3885 | −0.7842 |
| 18 | O | −2.2869 | −0.9619 | +3.5593 |
| 19 | Ca | +0.0000 | +0.0000 | −3.4214 |
| 20 | Ca | +0.0000 | +0.0000 | +0.0000 |
| 21 | Ca | +0.0000 | +0.0000 | +3.4214 |
| 22 | O | +2.2869 | +0.9619 | −3.5593 |
| 23 | Ca | +3.1622 | +1.3885 | +0.7842 |
| 24 | P(3) | −2.3334 | −1.3472 | +2.0654 |
| 25 | O | +1.5874 | +0.0439 | +1.6409 |
| 26 | O | −0.7557 | −1.3966 | +1.6409 |
| 27 | O | +3.0580 | +0.2203 | −1.1499 |
| 28 | O | −2.8378 | −2.7174 | +1.4609 |
| 29 | O | +0.8317 | −1.3528 | −1.6409 |
| 30 | O | −1.3382 | −2.7585 | −1.1499 |
| 31 | O | −0.3104 | −2.4615 | −3.5593 |
| 32 | O | +1.9765 | −1.4995 | +3.5593 |
| 33 | P(2) | +2.3334 | −1.3472 | +2.0654 |
| 34 | P(6) | +0.0000 | −2.6944 | −2.0654 |
| 35 | O | +3.7722 | −1.0989 | +1.4609 |
| 36 | Ca | −0.3786 | −3.4328 | +0.7842 |
| 37 | O | +1.7198 | −2.5381 | +1.1499 |
| 38 | Ca | +2.7835 | −2.0443 | −0.7842 |
| 39 | O | +0.9344 | −3.8163 | −1.4609 |
